# Supplementary material for: LogoRA: Local-Global Representation Alignment for Robust Time Series Classification
Source: arXiv:2409.12169 source file (2024-09-12)
Supplement: Supplementary file 1 [file appendix.tex]

\subsection{Cross Attention Between Global and Local feature in Fusion Module}
\label{sec:cross-attn}
% \begin{table}[t]
%     \centering
%     \caption{Comparison of various feature fusion methods}
%     \label{tab:cross-attn}
%     \begin{tabular}{c|ccc}
%     \toprule
%         source → target & addition & concatenation & cross attention \\
%         \midrule
%  0 → 2 & 0.6849 & 0.7857 & 0.8235 \\
%  1 → 6 & 0.8884 & 0.9163 & 0.9163 \\
%  2 → 4 & 0.4462 & 0.3386 & 0.9363 \\
%  4 → 0 & 0.2620 & 0.2576 & 0.3886 \\
%  4 → 1 & 0.6679 & 0.5672 & 0.9627 \\
%  5 → 1 & 0.8582 & 0.8694 & 0.9851 \\
%  7 → 1 & 0.8918 & 0.8545 & 0.9478 \\
%  7 → 5 & 0.4402 & 0.5637 & 0.8147 \\
%  8 → 3 & 0.8996 & 0.9738 & 0.9738 \\
%  8 → 4 & 0.6175 & 0.7331 & 0.9681 \\
%  \midrule
%  Avg & 0.6656 & 0.6860 & 0.8717  \\
%  \bottomrule
%     \end{tabular}
    
% \end{table}
Firstly, the cross-attention operation is able to extract useful robust context information between global and local features and is commonly used in other fields~\cite{Zhu_2022_CVPR}. Thanks to the modeling capability of Transformers for long dependencies, we extract the global features of the data and force the global features to be time-step invariant through DTW. The local features extracted by the convolutional network remain in temporal order, which can be matched with the patch-wise global feature. Moreover, a global feature summarizes the content of a sequence, often leading to a compact representation. Local features, on the other hand, comprise pattern information about specific regions, which are especially useful for classification. Generally speaking, global features are better at recall, while local features are better at precision~\cite{cao2020unifying}. So, we assume that local features with more relevant information to global features are more important. As shown in the heatmap in \figurename~\ref{fig:attn}, the higher the similarity calculated between global and local features, the more useful the corresponding part is for classification. Therefore, based on similarity score, further selecting local features can yield features that contain more useful contextual information. Besides, with different kernel sizes, we obtain several local features of different scale. So, using similarity score to select the multi-scale local feature helps to extract the effective features on different positions more comprehensively.
